# Supplementary material for: Reference Energies for Double Excitations: Improvement and Extension
Source: arXiv:2403.19597 ancillary file (2024-05-16)
Supplement: Supplementary file 1 [file supp.pdf]

# Supporting Information for "Reference Energies for Double Excitations: Improvement and Extension"

Fábris Kossoski,[1, a)] Martial Boggio-Pasqua,[1, b)] Pierre-François Loos,[1, c)] and Denis Jacquemin[2, 3, d)]
[1)] *Laboratoire de Chimie et Physique Quantiques (UMR 5626), Université de Toulouse, CNRS, UPS, France*
[2)] *Nantes Université, CNRS, CEISAM UMR 6230, F-44000 Nantes, France*
[3)] *Institut Universitaire de France (IUF), F-75005 Paris, France*

## S1. GEOMETRIES

Below are given the Cartesian coordinates for the compounds investigated in the present manuscript. These are provided in atomic units (bohr).

### Acrolein

Level of theory: CC3(Full)/*aug*-cc-pVTZ

```
C   -1.11645072          -0.68348783           0.00000000
C    1.20647847           0.83714564           0.00000000
C    3.46831059          -0.28872636           0.00000000
O   -3.23666415           0.19187203           0.00000000
H   -0.80613858          -2.74747338           0.00000000
H    0.98699813           2.86613511           0.00000000
H    5.20930864           0.77443560           0.00000000
H    3.60951559          -2.33000749           0.00000000
```

### Benzene

Level of theory: CC3(Full)/*aug*-cc-pVTZ

```
C    0.00000000           2.63144965           0.00000000
C   -2.27890225           1.31572483           0.00000000
C   -2.27890225          -1.31572483           0.00000000
C    0.00000000          -2.63144965           0.00000000
C    2.27890225          -1.31572483           0.00000000
C    2.27890225           1.31572483           0.00000000
H   -4.04725813           2.33668557           0.00000000
H   -4.04725813          -2.33668557           0.00000000
H   -0.00000000          -4.67337115           0.00000000
H    4.04725813          -2.33668557           0.00000000
H    4.04725813           2.33668557           0.00000000
H    0.00000000           4.67337115           0.00000000
```

### Benzoquinone

Level of theory: CC3(Full)/*aug*-cc-pVTZ

[a)] Electronic mail: fkossoski@irsamc.ups-tlse.fr
[b)] Electronic mail: martial.boggio@irsamc.ups-tlse.fr
[c)] Electronic mail: loos@irsamc.ups-tlse.fr
[d)] Electronic mail: Denis.Jacquemin@univ-nantes.fr

| | | | |
|---|---|---|---|
| C | 2.71467427 | 0.00000000 | 0.00000000 |
| C | -2.71467427 | 0.00000000 | 0.00000000 |
| C | 1.26645689 | 2.38719964 | 0.00000000 |
| C | 1.26645689 | -2.38719964 | 0.00000000 |
| C | -1.26645689 | 2.38719964 | 0.00000000 |
| C | -1.26645689 | -2.38719964 | 0.00000000 |
| O | 5.02607647 | 0.00000000 | 0.00000000 |
| O | -5.02607647 | 0.00000000 | 0.00000000 |
| H | 2.37218673 | 4.10318853 | 0.00000000 |
| H | 2.37218673 | -4.10318853 | 0.00000000 |
| H | -2.37218673 | 4.10318853 | 0.00000000 |
| H | -2.37218673 | -4.10318853 | 0.00000000 |

**Borole**

Level of theory: CC3(Full)/*aug*-cc-pVTZ

| | | | |
|---|---|---|---|
| B | 0.00000000 | 0.00000000 | 2.44991435 |
| C | 0.00000000 | 2.35991046 | 0.62561328 |
| C | 0.00000000 | -2.35991046 | 0.62561328 |
| C | 0.00000000 | 1.42526648 | -1.74135978 |
| C | 0.00000000 | -1.42526648 | -1.74135978 |
| H | 0.00000000 | 0.00000000 | 4.69246473 |
| H | 0.00000000 | 4.35732912 | 1.03002724 |
| H | 0.00000000 | -4.35732912 | 1.03002724 |
| H | 0.00000000 | 2.51021632 | -3.47247633 |
| H | 0.00000000 | -2.51021632 | -3.47247633 |

**Butadiene**

Level of theory: CC3(Full)/*aug*-cc-pVTZ

| | | | |
|---|---|---|---|
| C | 1.14656244 | 0.00000000 | 0.75468820 |
| C | -1.14656244 | 0.00000000 | -0.75468820 |
| C | 3.48132647 | 0.00000000 | -0.22482805 |
| C | -3.48132647 | 0.00000000 | 0.22482805 |
| H | 0.90770978 | 0.00000000 | 2.78883925 |
| H | -0.90770978 | 0.00000000 | -2.78883925 |
| H | 3.77525814 | 0.00000000 | -2.24895470 |
| H | -3.77525814 | 0.00000000 | 2.24895470 |
| H | 5.13664967 | 0.00000000 | 0.96861890 |
| H | -5.13664967 | 0.00000000 | -0.96861890 |

**Carbon dimer**

Level of theory: CC3(Full)/*aug*-cc-pVTZ

| | | | |
|---|---|---|---|
| C | 0.00000000 | 0.00000000 | 1.17922927 |
| C | 0.00000000 | 0.00000000 | -1.17922927 |

**Carbon trimer**

Level of theory: CC3(Full)/*aug*-cc-pVTZ

| | | | |
|---|---|---|---|
| C | 0.00000000 | 0.00000000 | 0.00000000 |
| C | 0.00000000 | 0.00000000 | 2.45345613 |
| C | 0.00000000 | 0.00000000 | -2.45345613 |

### Criegee's Intermediate

Level of theory: CC3(Full)/*aug*-cc-pVTZ

| | | | |
|---|---|---|---|
| C | -2.14193693 | 0.46449461 | 0.00000000 |
| O | -0.12214743 | -0.85046436 | 0.00000000 |
| O | 2.09779397 | 0.38347786 | 0.00000000 |
| H | -3.86593284 | -0.61908241 | 0.00000000 |
| H | -1.98533536 | 2.49983926 | 0.00000000 |

### Cyclobutadiene

Level of theory: CC3(Full)/*aug*-cc-pVTZ

| | | | |
|---|---|---|---|
| C | -1.47868321 | -1.27004715 | 0.00000000 |
| C | 1.47868321 | -1.27004715 | 0.00000000 |
| C | -1.47868321 | 1.27004715 | 0.00000000 |
| C | 1.47868321 | 1.27004715 | 0.00000000 |
| H | -2.91448237 | -2.70994518 | 0.00000000 |
| H | 2.91448237 | -2.70994518 | 0.00000000 |
| H | -2.91448237 | 2.70994518 | 0.00000000 |
| H | 2.91448237 | 2.70994518 | 0.00000000 |

### Cyclopentadiene

Level of theory: CC3(Full)/*aug*-cc-pVTZ

| | | | |
|---|---|---|---|
| C | 0.00000000 | 0.00000000 | -2.33113051 |
| C | 0.00000000 | 2.22209092 | -0.56871188 |
| C | 0.00000000 | -2.22209092 | -0.56871188 |
| C | 0.00000000 | 1.38514451 | 1.83772922 |
| C | 0.00000000 | -1.38514451 | 1.83772922 |
| H | 1.66130504 | 0.00000000 | -3.56414299 |
| H | -1.66130504 | 0.00000000 | -3.56414299 |
| H | 0.00000000 | 4.16550405 | -1.18116624 |
| H | 0.00000000 | -4.16550405 | -1.18116624 |
| H | 0.00000000 | 2.54514584 | 3.51352303 |
| H | 0.00000000 | -2.54514584 | 3.51352303 |

### Cyclopentadienethione

Level of theory: CC3(Full)/*aug*-cc-pVTZ

| | | | |
|---|---|---|---|
| C | 0.00000000 | 0.00000000 | 0.54718884 |
| C | 0.00000000 | 2.23394142 | -1.11648863 |
| C | 0.00000000 | -2.23394142 | -1.11648863 |
| C | 0.00000000 | 1.40618242 | -3.52381930 |
| C | 0.00000000 | -1.40618242 | -3.52381930 |
| S | 0.00000000 | 0.00000000 | 3.63323789 |
| H | 0.00000000 | 4.14572930 | -0.42732005 |
| H | 0.00000000 | -4.14572930 | -0.42732005 |

| | | | |
|---|---|---|---|
| H | 0.00000000 | 2.55090221 | -5.20908210 |
| H | 0.00000000 | -2.55090221 | -5.20908210 |

**Cyclopentadienone**

Level of theory: CC3(Full)/*aug*-cc-pVTZ

| | | | |
|---|---|---|---|
| C | 0.00000000 | 0.00000000 | 1.45232781 |
| C | 0.00000000 | 2.26718523 | -0.25413145 |
| C | 0.00000000 | -2.26718523 | -0.25413145 |
| C | 0.00000000 | 1.41557636 | -2.63852689 |
| C | 0.00000000 | -1.41557636 | -2.63852689 |
| O | 0.00000000 | 0.00000000 | 3.74438847 |
| H | 0.00000000 | 4.18416912 | 0.42151096 |
| H | 0.00000000 | -4.18416912 | 0.42151096 |
| H | 0.00000000 | 2.53760914 | -4.33851399 |
| H | 0.00000000 | -2.53760914 | -4.33851399 |

**Diazete**

Level of theory: CC3(Full)/*aug*-cc-pVTZ

| | | | |
|---|---|---|---|
| C | 1.04088890 | 1.37023206 | 0.00000000 |
| C | -1.04088890 | -1.37023206 | 0.00000000 |
| N | 1.80420222 | -0.93584807 | 0.00000000 |
| N | -1.80420222 | 0.93584807 | 0.00000000 |
| H | 2.06402011 | 3.13844681 | 0.00000000 |
| H | -2.06402011 | -3.13844681 | 0.00000000 |

**Ethylene**

Level of theory: CC3(Full)/*aug*-cc-pVTZ

| | | | |
|---|---|---|---|
| C | 0.00000000 | 1.26026583 | 0.00000000 |
| C | 0.00000000 | -1.26026583 | 0.00000000 |
| H | 0.00000000 | 2.32345976 | 1.74287672 |
| H | 0.00000000 | -2.32345976 | 1.74287672 |
| H | 0.00000000 | 2.32345976 | -1.74287672 |
| H | 0.00000000 | -2.32345976 | -1.74287672 |

**Formaldehyde**

Level of theory: CC3(Full)/*aug*-cc-pVTZ

| | | | |
|---|---|---|---|
| C | 0.00000000 | 0.00000000 | -1.13947666 |
| O | 0.00000000 | 0.00000000 | 1.14402883 |
| H | 0.00000000 | 1.76627623 | -2.23398653 |
| H | 0.00000000 | -1.76627623 | -2.23398653 |

**Glyoxal**

Level of theory: CC3(Full)/*aug*-cc-pVTZ

| | | | |
|---|---|---|---|
| C | 1.21360282 | 0.75840215 | 0.00000000 |
| C | -1.21360282 | -0.75840215 | 0.00000000 |
| O | 3.25581408 | -0.26453186 | 0.00000000 |
| O | -3.25581408 | 0.26453186 | 0.00000000 |
| H | 0.96135276 | 2.81883243 | 0.00000000 |
| H | -0.96135276 | -2.81883243 | 0.00000000 |

**Hexatriene**

Level of theory: CC3(Full)/*aug*-cc-pVTZ

| | | | |
|---|---|---|---|
| C | 1.14024826 | 0.56596845 | 0.00000000 |
| C | -1.14024826 | -0.56596845 | 0.00000000 |
| C | 3.51540649 | -0.78907931 | 0.00000000 |
| C | -3.51540649 | 0.78907931 | 0.00000000 |
| C | 5.78668151 | 0.33754155 | 0.00000000 |
| C | -5.78668151 | -0.33754155 | 0.00000000 |
| H | 1.23448067 | 2.61584039 | 0.00000000 |
| H | -1.23448067 | -2.61584039 | 0.00000000 |
| H | 3.40773630 | -2.83459321 | 0.00000000 |
| H | -3.40773630 | 2.83459321 | 0.00000000 |
| H | 5.95047109 | 2.37626316 | 0.00000000 |
| H | -5.95047109 | -2.37626316 | 0.00000000 |
| H | 7.51470672 | -0.74809921 | 0.00000000 |
| H | -7.51470672 | 0.74809921 | 0.00000000 |

**Naphthalene**

Level of theory: CC3(Full)/cc-pVTZ

| | | | |
|---|---|---|---|
| C | 0.00000000 | 1.33999524 | 0.00000000 |
| C | 0.00000000 | -1.33999524 | 0.00000000 |
| C | 2.33779858 | 2.63841577 | 0.00000000 |
| C | -2.33779858 | 2.63841577 | 0.00000000 |
| C | 2.33779858 | -2.63841577 | 0.00000000 |
| C | -2.33779858 | -2.63841577 | 0.00000000 |
| C | 4.57964958 | 1.33587048 | 0.00000000 |
| C | -4.57964958 | 1.33587048 | 0.00000000 |
| C | 4.57964958 | -1.33587048 | 0.00000000 |
| C | -4.57964958 | -1.33587048 | 0.00000000 |
| H | 2.32888235 | 4.67949410 | 0.00000000 |
| H | -2.32888235 | 4.67949410 | 0.00000000 |
| H | 2.32888235 | -4.67949410 | 0.00000000 |
| H | -2.32888235 | -4.67949410 | 0.00000000 |
| H | 6.34884007 | 2.34551705 | 0.00000000 |
| H | -6.34884007 | 2.34551705 | 0.00000000 |
| H | 6.34884007 | -2.34551705 | 0.00000000 |
| H | -6.34884007 | -2.34551705 | 0.00000000 |

**Nitrosomethane**

Level of theory: CC3(Full)/*aug*-cc-pVTZ

| | | | |
|---|---|---|---|
| C | -1.78426612 | 0.00000000 | -1.07224050 |
| N | -0.00541753 | 0.00000000 | 1.08060391 |
| O | 2.18814985 | 0.00000000 | 0.43452135 |

| | | | |
|---|---|---|---|
| H | -0.77343975 | 0.00000000 | -2.86415606 |
| H | -2.97471478 | 1.66801808 | -0.86424584 |
| H | -2.97471478 | -1.66801808 | -0.86424584 |

**Nitrous acid**

Level of theory: CC3(FC)/*aug*-cc-pVTZ

| | | | |
|---|---|---|---|
| H | -3.27788005 | 0.93588010 | 0.00000000 |
| N | 0.29308547 | 0.93895729 | 0.00000000 |
| O | -2.05678600 | -0.42335161 | 0.00000000 |
| O | 2.00673459 | -0.45764664 | 0.00000000 |

**Nitroxyl**

Level of theory: CC3(Full)/*aug*-cc-pVTZ

| | | | |
|---|---|---|---|
| O | 0.21099695 | 0.00000000 | 2.15462460 |
| N | -0.44776863 | 0.00000000 | -0.03589263 |
| H | 1.18163475 | 0.00000000 | -1.17386890 |

**Octatetraene**

Level of theory: CC3(Full)/cc-pVTZ

| | | | |
|---|---|---|---|
| C | 1.19649232 | 0.64794934 | 0.00000000 |
| C | -1.19649232 | -0.64794934 | 0.00000000 |
| C | 3.45745137 | -0.52964709 | 0.00000000 |
| C | -3.45745137 | 0.52964709 | 0.00000000 |
| C | 5.85705040 | 0.77625595 | 0.00000000 |
| C | -5.85705040 | -0.77625595 | 0.00000000 |
| C | 8.10525884 | -0.39700663 | 0.00000000 |
| C | -8.10525884 | 0.39700663 | 0.00000000 |
| H | 1.14813002 | 2.69304901 | 0.00000000 |
| H | -1.14813002 | -2.69304901 | 0.00000000 |
| H | 3.50962357 | -2.57436634 | 0.00000000 |
| H | -3.50962357 | 2.57436634 | 0.00000000 |
| H | 5.78969253 | 2.81832245 | 0.00000000 |
| H | -5.78969253 | -2.81832245 | 0.00000000 |
| H | 8.22516217 | -2.43500100 | 0.00000000 |
| H | -8.22516217 | 2.43500100 | 0.00000000 |
| H | 9.85247043 | 0.65022932 | 0.00000000 |
| H | -9.85247043 | -0.65022932 | 0.00000000 |

**Oxalyl fluoride**

Level of theory: CC3(Full)/*aug*-cc-pVTZ

| | | | |
|---|---|---|---|
| C | -1.39903565 | 0.34476183 | 0.00000000 |
| C | 1.39903565 | -0.34476183 | 0.00000000 |
| O | -2.24825627 | 2.40855549 | 0.00000000 |
| O | 2.24825627 | -2.40855549 | 0.00000000 |
| F | -2.78737061 | -1.74488227 | 0.00000000 |
| F | 2.78737061 | 1.74488227 | 0.00000000 |

### Pyrazine

Level of theory: CC3(Full)/*aug*-cc-pVTZ

| | | | |
|---|---|---|---|
| C | 0.00000000 | 2.13188686 | 1.31510863 |
| C | 0.00000000 | -2.13188686 | 1.31510863 |
| C | 0.00000000 | 2.13188686 | -1.31510863 |
| C | 0.00000000 | -2.13188686 | -1.31510863 |
| N | 0.00000000 | 0.00000000 | 2.66620111 |
| N | 0.00000000 | 0.00000000 | -2.66620111 |
| H | 0.00000000 | 3.88751412 | 2.35234226 |
| H | 0.00000000 | -3.88751412 | 2.35234226 |
| H | 0.00000000 | 3.88751412 | -2.35234226 |
| H | 0.00000000 | -3.88751412 | -2.35234226 |

### Tetrazine

Level of theory: CC3(Full)/*aug*-cc-pVTZ

| | | | |
|---|---|---|---|
| C | 0.00000000 | 0.00000000 | 2.38208164 |
| C | 0.00000000 | 0.00000000 | -2.38208164 |
| N | 2.25673244 | 0.00000000 | 1.24973261 |
| N | -2.25673244 | 0.00000000 | 1.24973261 |
| N | 2.25673244 | 0.00000000 | -1.24973261 |
| N | -2.25673244 | 0.00000000 | -1.24973261 |
| H | 0.00000000 | 0.00000000 | 4.41850901 |
| H | 0.00000000 | 0.00000000 | -4.41850901 |

## S2. ADDITIONAL FIGURES AND TABLES

Here, we include, for the various CC and multiconfigurational methods considered here, the MAEs for the excitation energies, the MAEs for the basis set effect, the errors of the basis set effects as functions of $\%T_1$, and the distribution of errors on the excitation energies.

TABLE S1. Mean absolute error (MAE), in units of eV, with respect to the TBEs, for various bare CC and multiconfigurational methods and their +LT1 analogs (discussed in the main text), including all excitations labeled as safe, and the subsets of genuine and partial doubly-excited states, while accounting for the three basis sets.

| Method | # | bare | +LT1 |
|---|---|---|---|
| | All safe excitations | | |
| CCSDTQ | 39 | 0.03 | 0.02 |
| CC4 | 48 | 0.05 | 0.03 |
| CCSDT | 60 | 0.27 | 0.14 |
| CC3 | 63 | 0.53 | 0.16 |
| CASPT2(IPEA) | 63 | 0.12 | 0.12 |
| CASPT3(IPEA) | 63 | 0.13 | 0.09 |
| CASPT3 | 63 | 0.11 | 0.09 |
| SC-NEVPT2 | 63 | 0.15 | 0.11 |
| PC-NEVPT2 | 63 | 0.13 | 0.12 |
| | Genuine doubly-excited states | | |
| CCSDTQ | 28 | 0.04 | 0.03 |
| CC4 | 28 | 0.08 | 0.05 |
| CCSDT | 33 | 0.42 | 0.21 |
| CC3 | 33 | 0.90 | 0.27 |
| CASPT2(IPEA) | 33 | 0.12 | 0.13 |
| CASPT3(IPEA) | 33 | 0.08 | 0.07 |
| CASPT3 | 33 | 0.08 | 0.08 |
| SC-NEVPT2 | 33 | 0.09 | 0.08 |
| PC-NEVPT2 | 33 | 0.09 | 0.09 |
| | Partial doubly-excited states | | |
| CCSDTQ | 11 | 0.00 | 0.00 |
| CC4 | 20 | 0.01 | 0.01 |
| CCSDT | 27 | 0.09 | 0.06 |
| CC3 | 30 | 0.13 | 0.04 |
| CASPT2(IPEA) | 30 | 0.13 | 0.10 |
| CASPT3(IPEA) | 30 | 0.19 | 0.11 |
| CASPT3 | 30 | 0.14 | 0.09 |
| SC-NEVPT2 | 30 | 0.21 | 0.15 |
| PC-NEVPT2 | 30 | 0.17 | 0.16 |

TABLE S2. Mean absolute error (MAE) on the basis set effect, in units of eV, with respect to the TBE reference values, for the three basis set differences, AVDZ − Pop, AVTZ − AVDZ, and AVTZ − Pop, computed for the various CC and multiconfigurational methods, including all excitations labeled as safe, and the subsets of genuine and partial doubly-excited states. Ethylene is excluded from the statistics for the multiconfigurational methods.

| Method | AVDZ − Pop | AVTZ − AVDZ | AVTZ − Pop |
|---|---|---|---|
| | All safe excitations | | |
| CCSDTQ | 0.003 | 0.007 | 0.009 |
| CC4 | 0.009 | 0.016 | 0.006 |
| CCSDT | 0.021 | 0.047 | 0.071 |
| CC3 | 0.046 | 0.032 | 0.076 |
| CASPT2(IPEA) | 0.034 | 0.030 | 0.022 |
| CASPT3(IPEA) | 0.030 | 0.021 | 0.017 |
| CASPT3 | 0.025 | 0.019 | 0.018 |
| SC-NEVPT2 | 0.035 | 0.028 | 0.028 |
| PC-NEVPT2 | 0.032 | 0.029 | 0.030 |
| | Genuine doubly-excited states | | |
| CCSDTQ | 0.002 | 0.008 | 0.010 |
| CC4 | 0.014 | 0.021 | 0.006 |
| CCSDT | 0.038 | 0.076 | 0.113 |
| CC3 | 0.075 | 0.054 | 0.126 |
| CASPT2(IPEA) | 0.024 | 0.022 | 0.024 |
| CASPT3(IPEA) | 0.015 | 0.018 | 0.011 |
| CASPT3 | 0.013 | 0.018 | 0.015 |
| SC-NEVPT2 | 0.016 | 0.024 | 0.027 |
| PC-NEVPT2 | 0.013 | 0.025 | 0.031 |
| | Partial doubly-excited states | | |
| CCSDTQ | 0.004 | 0.002 | 0.003 |
| CC4 | 0.002 | 0.001 | 0.006 |
| CCSDT | 0.003 | 0.001 | 0.004 |
| CC3 | 0.013 | 0.008 | 0.022 |
| CASPT2(IPEA) | 0.045 | 0.037 | 0.019 |
| CASPT3(IPEA) | 0.044 | 0.025 | 0.023 |
| CASPT3 | 0.037 | 0.021 | 0.021 |
| SC-NEVPT2 | 0.054 | 0.032 | 0.030 |
| PC-NEVPT2 | 0.052 | 0.033 | 0.028 |

TABLE S3. Values of the parameters $a$ and $b$ (in eV), obtained by fitting a linear function $a \times \%T_1/100 + b$, to the error on the excitation energies (with respect to our theoretical best estimates) against the $\%T_1$ value obtained at the CC3/aug-cc-pVTZ level of theory. The data for the three basis sets and for both safe and unsafe states are taken into account for the fitting.

| Method | $a$ | $b$ |
|---|---|---|
| CC3 | −1.2286 | 1.1127 |
| CCSDT | −0.6831 | 0.6518 |
| CC4 | −0.0903 | 0.0676 |
| CCSDTQ | −0.0530 | 0.0383 |
| CASPT2(IPEA) | 0.1960 | −0.0326 |
| CASPT3(IPEA) | 0.1479 | 0.0593 |
| CASPT3 | 0.0764 | 0.0465 |
| SC-NEVTP2 | 0.2861 | 0.0132 |
| PC-NEVTP2 | 0.2400 | −0.0081 |

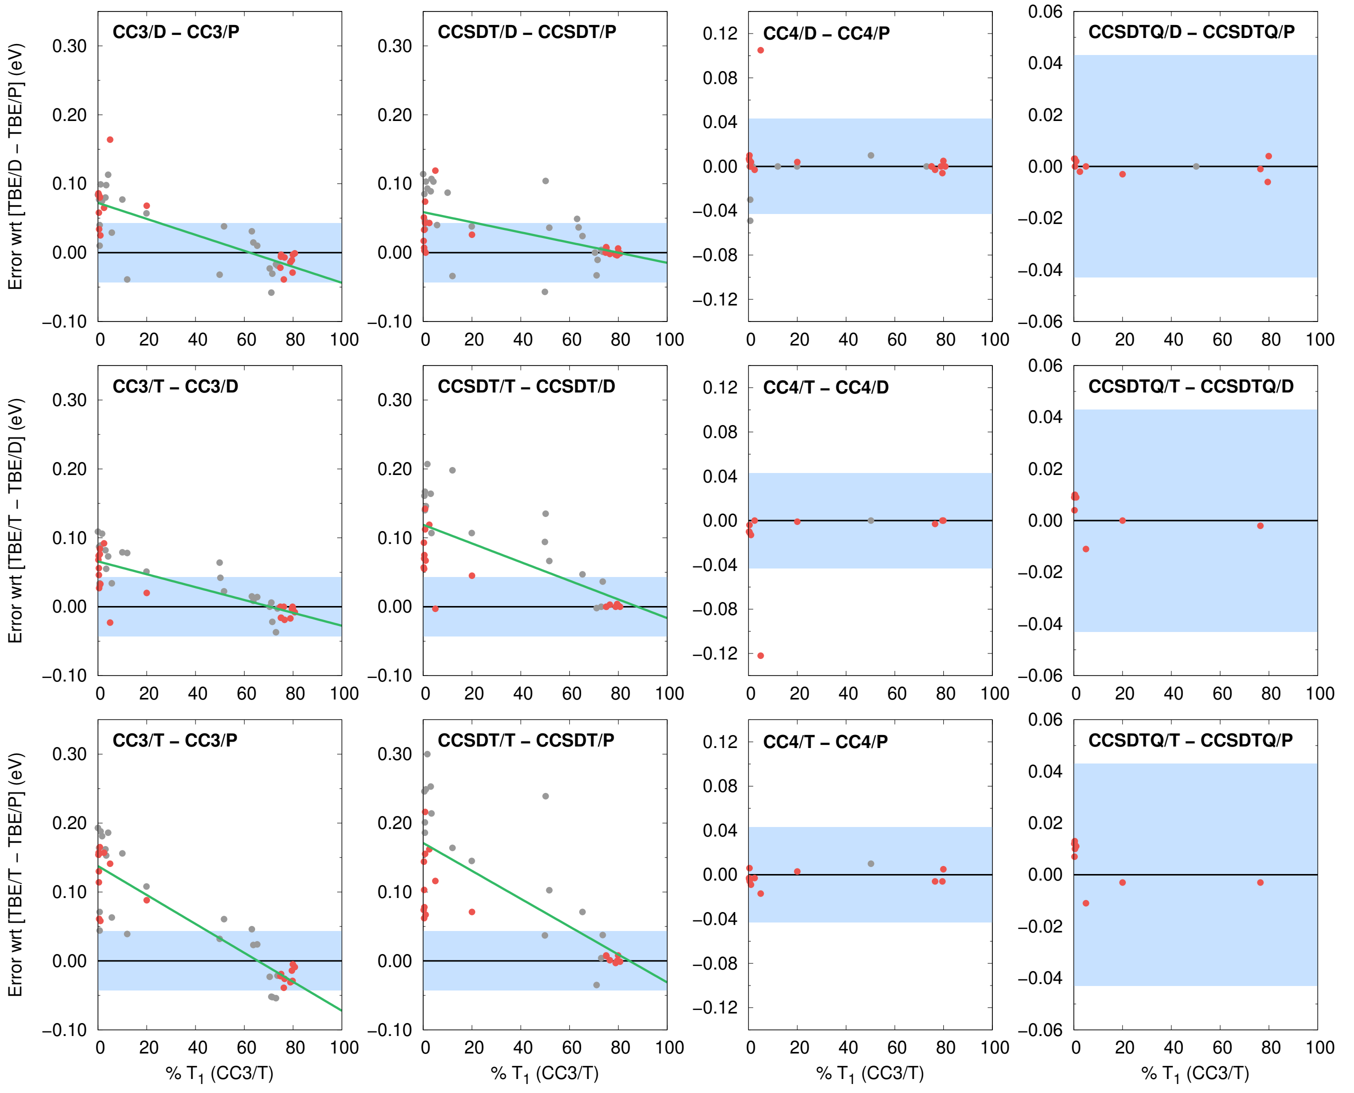


FIG. S1. Errors on the basis set effect (with respect to the TBE values), for various CC methods, as functions of the $\%T_1$ value obtained from CC3/AVTZ calculations, for both safe (red) and unsafe (gray) states. A linear fit to both safe and unsafe data points is shown as a green line, whereas chemical accuracy (0.043 eV) is represented by the blue region. For the sake of conciseness, the 6-31+G(d), aug-cc-pVDZ, and aug-cc-pVTZ basis sets are labeled P, D, and T, respectively.

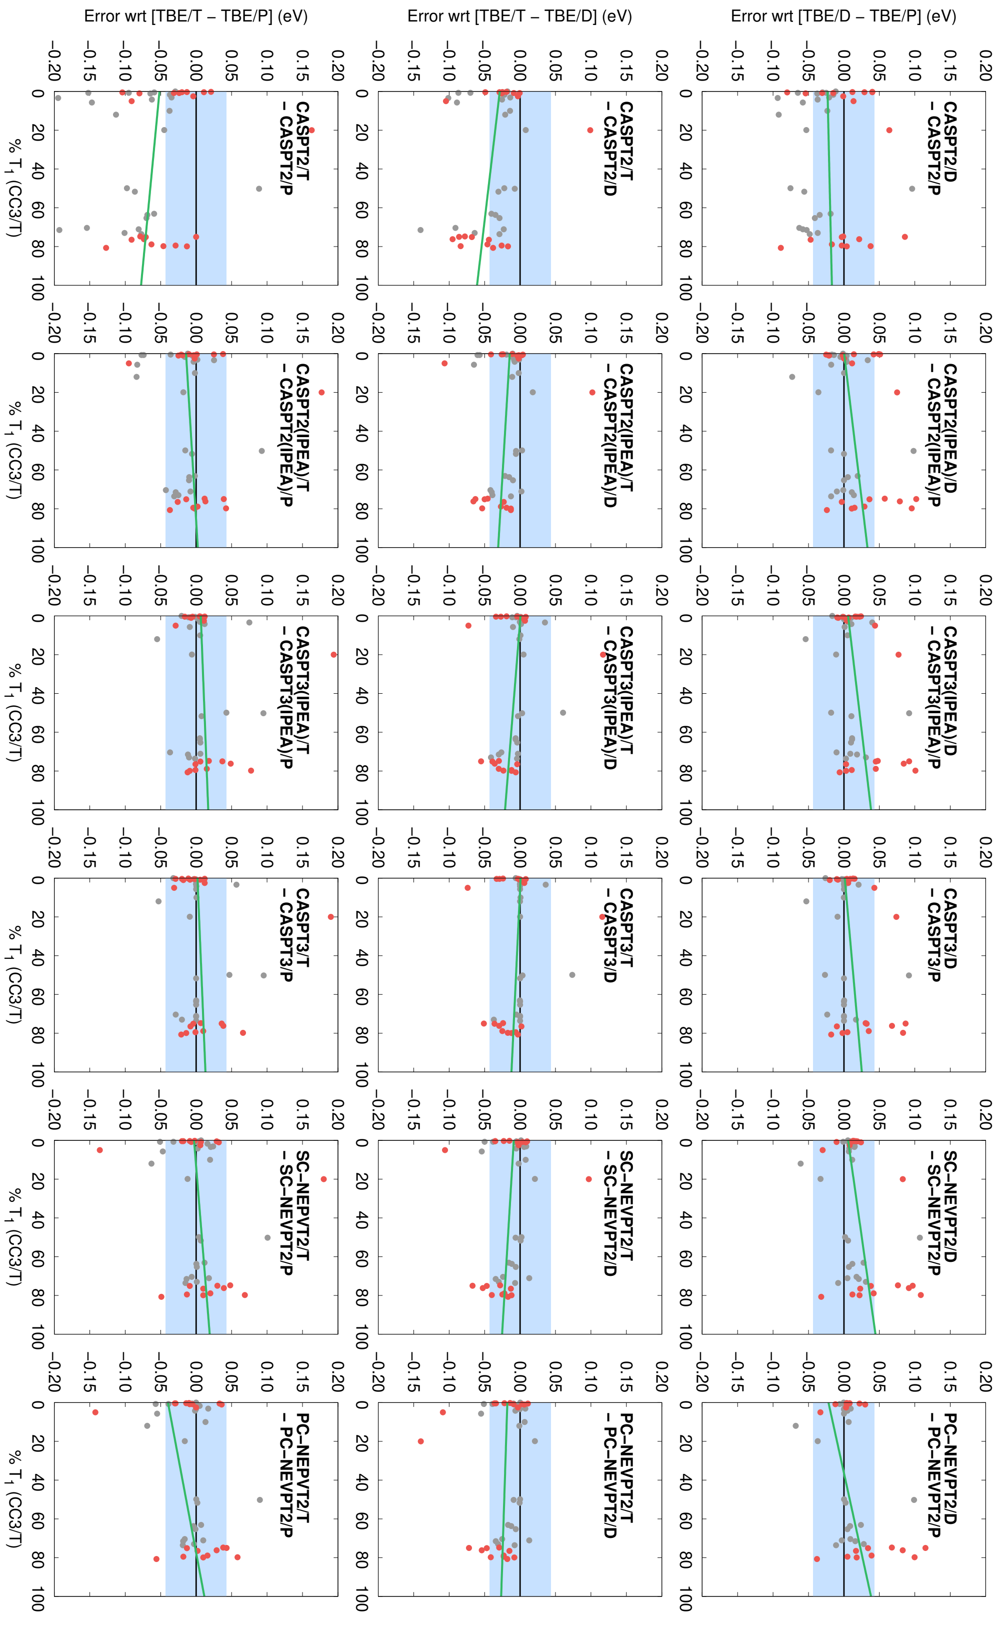


FIG. S2. Errors on the basis set effect (with respect to the TBE values), for various multiconfigurational methods, as functions of the $\%T_1$ value obtained from CC3/AVTZ calculations, for both safe (red) and unsafe (gray) states. A linear fit to both safe and unsafe data points is shown as a green line, whereas chemical accuracy (0.043 eV) is represented by the blue region. For the sake of conciseness, the 6-31+G(d), aug-cc-pVDZ, and aug-cc-pVTZ basis sets are labeled P, D, and T, respectively.

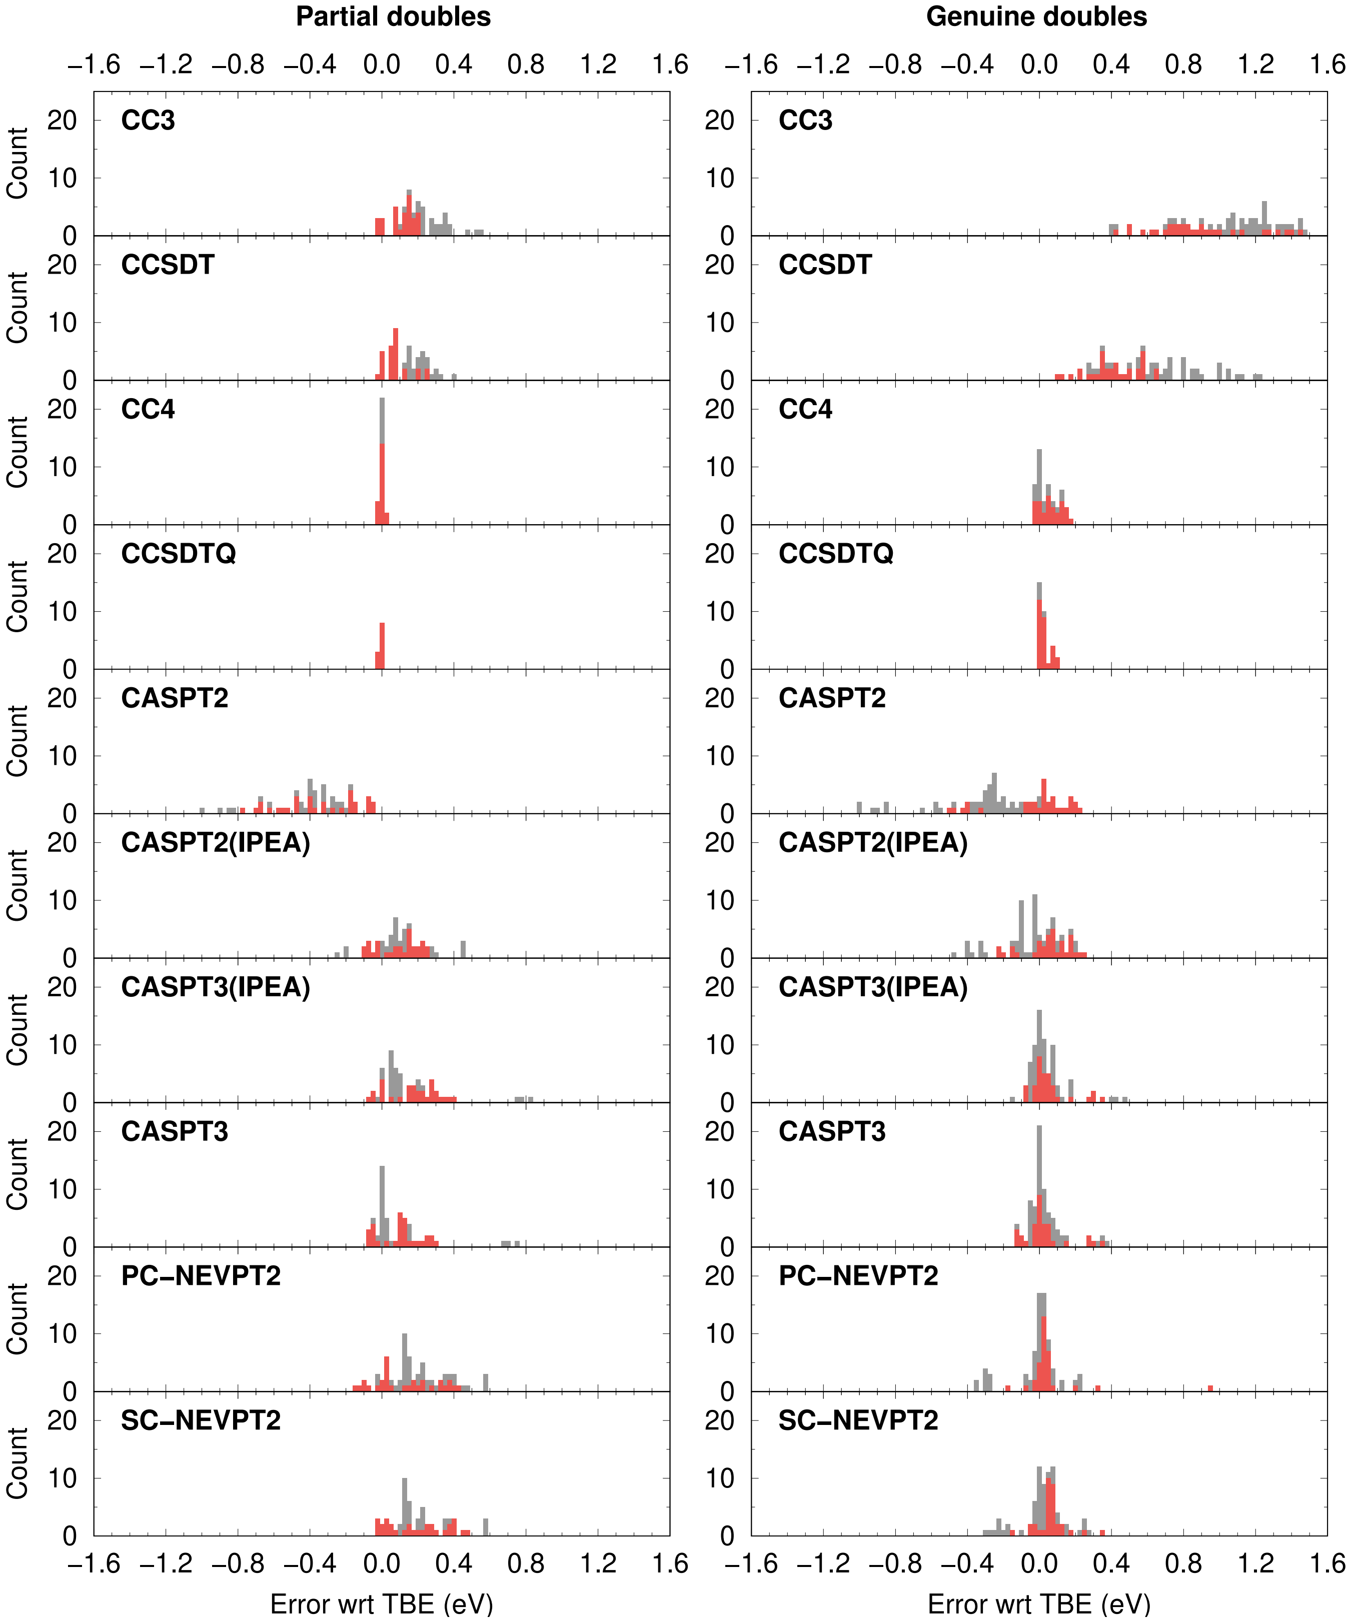


FIG. S3. Distribution of errors (with respect to the TBEs) on the excitation energies of partial (left) and genuine (right) doubly-excited states, for the various CC and multiconfigurational methods, including the three basis sets, and separated by safe (red) and unsafe (gray) states.

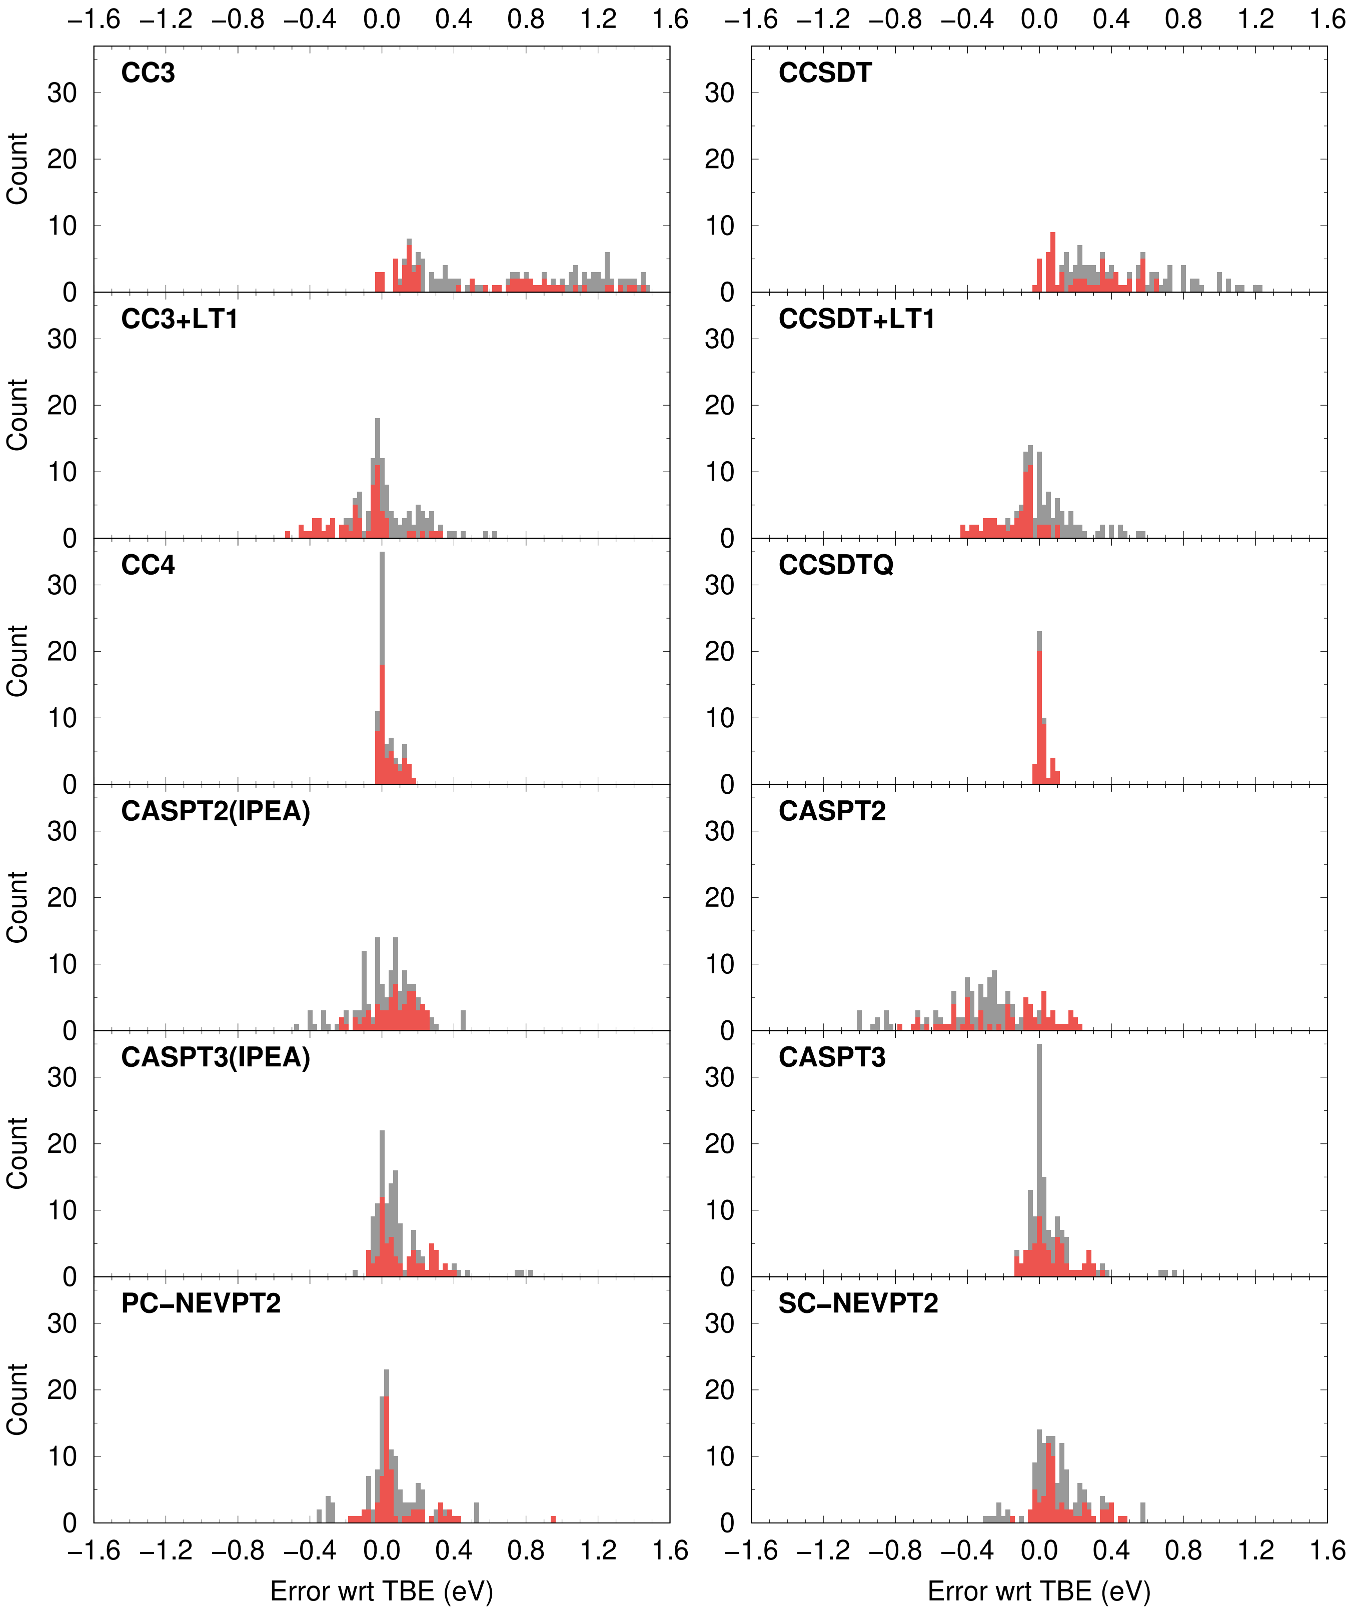


FIG. S4. Distribution of errors (with respect to the TBEs) on the excitation energies of both partial and genuine doubly-excited states, for the various CC and multiconfigurational methods, including the three basis sets, and separated by safe (red) and unsafe (gray) states.
