# Supplementary material for: Reference Energies for Double Excitations: Improvement and Extension
Source: arXiv:2403.19597 ancillary file (2024-05-16)
Supplement: Supplementary file 2 [file supp_tables_mrpt.pdf]

**Table S4.** CASSCF, CASPT2, NEVPT2 and CASPT3/aug-cc-pVTZ vertical transition energies (eV) of acrolein.

| State | Active space[a] (a',a") | State-average (A',A") | CASSCF | CASPT2 IPEA | CASPT2 NOIPEA | PC-NEVPT2 | SC-NEVPT2 | CASPT3 IPEA | CASPT3 NOIPEA |
|---|---|---|---|---|---|---|---|---|---|
| $^1A'(\pi-\pi^*)$ | (6,4) | (3,0) | 8.454 | **7.961** | **7.528** | **7.846** | **8.006** | **7.979** | **7.906** |

[a] Using reference (10e,10o) active space including valence $\pi$, $\sigma_{CC}$, $\sigma_{CO}$, $\sigma^*_{CC}$, $\sigma^*_{CO}$ orbitals.

**Table S5.** CASSCF, CASPT2, NEVPT2 and CASPT3/aug-cc-pVTZ vertical transition energies (eV) of benzene.

| State | Active space[a] ($a_g$,$b_{3u}$,$b_{2u}$,$b_{1g}$,$b_{1u}$,$b_{2g}$,$b_{3g}$,$a_u$) | State-average ($A_g$,$B_{3u}$,$B_{2u}$,$B_{1g}$,$B_{1u}$,$B_{2g}$,$B_{3g}$,$A_u$) | CASSCF | CASPT2 IPEA | CASPT2 NOIPEA | PC-NEVPT2 | SC-NEVPT2 | CASPT3 IPEA | CASPT3 NOIPEA |
|---|---|---|---|---|---|---|---|---|---|
| $^1E_{2g}(\pi-\pi^*)$ | (0,0,0,0,2,1,2,1) | (2,0,0,1,0,0,0,0) | 8.103 | **8.314** | **7.816**[b] | **8.512** | **8.555** | **8.263** | **8.162**[b] |
| $^1A_{1g}(\pi,\pi-\pi^*,\pi^*)$ | (0,0,0,0,2,1,2,1) | (3,0,0,1,0,0,0,0) | 11.444 | **10.236** | **9.326**[b] | **9.995** | **10.381** | **10.468** | **10.315**[b] |

[a] Using reference (6e,6o) active space including valence $\pi$ orbitals. [b] Level shift = 0.4 au.

**Table S6.** CASSCF, CASPT2, NEVPT2 and CASPT3/aug-cc-pVTZ vertical transition energies (eV) of benzoquinone.

| State | Active space ($a_g$,$b_{3u}$,$b_{2u}$,$b_{1g}$,$b_{1u}$,$b_{2g}$,$b_{3g}$,$a_u$) | State-average ($A_g$,$B_{3u}$,$B_{2u}$,$B_{1g}$,$B_{1u}$,$B_{2g}$,$B_{3g}$,$A_u$) | CASSCF | CASPT2 IPEA | CASPT2 NOIPEA | PC-NEVPT2 | SC-NEVPT2 | CASPT3 IPEA | CASPT3 NOIPEA |
|---|---|---|---|---|---|---|---|---|---|
| $^1A_g(\pi,\pi-\pi^*,\pi^*)$ | (0,0,1,1,3,3,1,1)[a] | (2,0,0,0,0,0,0,0) | 4.945 | **4.472** | **4.301** | **4.566** | **4.565** | **4.672** | **4.696** |
| $^1B_{2g}(n-\pi^*)$ | (0,0,1,1,3,3,1,1)[a] | (1,0,0,0,0,1,0,0) | 6.539 | **5.761** | **5.005**[b] | **5.932** | **6.004** | **6.028** | **5.950**[c] |
| $^1B_{1u}(n-\pi^*)$[c] | (0,0,1,1,3,3,1,1)[a] | (1,0,0,0,1,0,0,0) | 6.543 | **5.774** | **5.002**[b] | **5.944** | **6.020** | **6.036** | **5.954**[c] |
| $^1A_g(\pi-\pi^*)$ | (0,0,0,0,3,3,1,1)[d] | (2,0,0,0,0,0,0,0) | 6.526 | **6.287** | **5.849** | **6.390** | **6.431** | **6.343** | **6.303** |
| $^1A_u(n-\pi^*)$ | (0,0,1,1,3,3,1,1)[a] | (1,0,0,0,0,0,0,2) | 6.684 | **6.210** | **5.547**[b] | **6.502** | **6.548** | **6.422** | **6.352**[c] |
| $^1B_{3g}(n-\pi^*)$[e] | (0,0,1,1,3,3,1,1)[a] | (1,0,0,0,0,0,2,0) | 6.697 | **6.234** | **5.479**[b] | **6.530** | **6.574** | **6.451** | **6.492**[c] |

[a] Using reference (12e,10o) active space including valence $\pi$ and the two $n_O$ orbitals. [b] Level shift = 0.4 au. [c] Denoted $^1B_{3u}$ in article using a different symmetry convention. [d] Using reference (8e,8o) active space including valence $\pi$ orbitals. [e] Denoted $^1B_{1g}$ in article using a different symmetry convention.

**Table S7.** CASSCF, CASPT2, NEVPT2 and CASPT3/aug-cc-pVTZ vertical transition energies (eV) of beryllium.

| State | Active space[a] ($a_g$,$b_{3u}$,$b_{2u}$,$b_{1g}$,$b_{1u}$,$b_{2g}$,$b_{3g}$,$a_u$) | State-average ($A_g$,$B_{3u}$,$B_{2u}$,$B_{1g}$,$B_{1u}$,$B_{2g}$,$B_{3g}$,$A_u$) | CASSCF | CASPT2 IPEA | CASPT2 NOIPEA | PC-NEVPT2 | SC-NEVPT2 | CASPT3 IPEA | CASPT3 NOIPEA |
|---|---|---|---|---|---|---|---|---|---|
| $^1D(2s,2s-2p,2p)$ | (3,2,2,1,2,1,1,0) | (3,0,0,0,0,0,0,0) | 7.115 | **7.137** | **7.129** | **7.133** | **7.133** | **7.142** | **7.139** |

[a] Using reference (2e,12o) active space including full valence space plus 3p and 3d orbitals.

**Table S8.** CASSCF, CASPT2, NEVPT2 and CASPT3/aug-cc-pVTZ vertical transition energies (eV) of borole.

| State | Active space[a] ($a_1,b_1,b_2,a_2$) | State-average ($A_1,B_1,B_2,A_2$) | CASSCF | CASPT2 IPEA | CASPT2 NOIPEA | PC-NEVPT2 | SC-NEVPT2 | CASPT3 IPEA | CASPT3 NOIPEA |
|---|---|---|---|---|---|---|---|---|---|
| $^1A_1(\pi,\pi\text{-}\pi^*,\pi^*)$ | (0,3,0,2) | (2,0,0,0) | 5.013 | **4.798** | **4.580** | **4.760** | **4.785** | **4.792** | **4.753** |
| $^1A_1(\pi\text{-}\pi^*)$ | (0,3,0,2) | (3,0,0,0) | 7.814 | **6.650** | **5.979** | **6.368** | **6.484** | **6.760** | **6.622** |

[a] Using reference (4e,5o) active space including valence $\pi$ orbitals.

**Table S9.** CASSCF, CASPT2, NEVPT2 and CASPT3/aug-cc-pVTZ vertical transition energies (eV) of butadiene.

| State | Active space[a] ($a_g,a_u,b_u,b_g$) | State-average ($A_g,A_u,B_u,B_g$) | CASSCF | CASPT2 IPEA | CASPT2 NOIPEA | PC-NEVPT2 | SC-NEVPT2 | CASPT3 IPEA | CASPT3 NOIPEA |
|---|---|---|---|---|---|---|---|---|---|
| $^1A_g(\pi\text{-}\pi^*)$ | (3,2,3,2) | (2,0,0,0) | 6.990 | **6.736** | **6.384**[b] | **6.700** | **6.780** | **6.718** | **6.627**[b] |

[a] Using reference (10e,10o) active space including valence $\pi$, $\sigma_{CC}$, $\sigma^*_{CC}$ orbitals. [b] Level shift = 0.4 au.

**Table S10.** CASSCF, CASPT2, NEVPT2 and CASPT3/aug-cc-pVTZ vertical transition energies (eV) of carbon dimer.

| State | Active space[a] ($a_g,b_{3u},b_{2u},b_{1g},b_{1u},b_{2g},b_{3g},a_u$) | State-average ($A_g,B_{3u},B_{2u},B_{1g},B_{1u},B_{2g},B_{3g},A_u$) | CASSCF | CASPT2 IPEA | CASPT2 NOIPEA | PC-NEVPT2 | SC-NEVPT2 | CASPT3 IPEA | CASPT3 NOIPEA |
|---|---|---|---|---|---|---|---|---|---|
| $^1\Delta_g(\pi,\pi\text{-}\sigma^*,\sigma^*)$ | (2,1,1,0,2,1,1,0) | (2,0,0,1,0,0,0,0) | 2.487 | **2.271** | **2.277** | **2.119** | **2.144** | **2.126** | **2.096** |
| $^1\Sigma^+_g(\pi,\pi\text{-}\sigma^*,\sigma^*)$ | (2,1,1,0,2,1,1,0) | (2,0,0,0,0,0,0,0) | 2.842 | **2.558** | **2.518** | **2.423** | **2.478** | **2.439** | **2.397** |
| $^3\Sigma^-_g(\pi,\pi\text{-}\sigma^*,\sigma^*)$ | (2,1,1,0,2,1,1,0) | (1,0,0,1,0,0,0,0) | 1.742 | **1.476** | **1.461** | **1.266** | **1.328** | **1.318** | **1.279** |

[a] Using reference (8e,8o) active space including full valence space.

**Table S11.** CASSCF, CASPT2, NEVPT2 and CASPT3/aug-cc-pVTZ vertical transition energies (eV) of carbon trimer.

| State | Active space[a] ($a_g,b_{3u},b_{2u},b_{1g},b_{1u},b_{2g},b_{3g},a_u$) | State-average ($A_g,B_{3u},B_{2u},B_{1g},B_{1u},B_{2g},B_{3g},A_u$) | CASSCF | CASPT2 IPEA | CASPT2 NOIPEA | PC-NEVPT2 | SC-NEVPT2 | CASPT3 IPEA | CASPT3 NOIPEA |
|---|---|---|---|---|---|---|---|---|---|
| $^1\Pi_g(n\text{-}\pi^*)$ | (3,2,2,0,3,1,1,0) | (1,0,0,0,0,1,1,0) | 4.109 | **3.934** | **3.654** | **4.027** | **4.063** | **4.009** | **3.969** |
| $^1\Delta_g(n,n\text{-}\pi^*,\pi^*)$ | (3,2,2,0,3,1,1,0) | (2,0,0,1,0,0,0,0) | 4.985 | **5.027** | **4.744**[b] | **5.255** | **5.209** | **5.172** | **5.123**[b] |
| $^1\Sigma^+_g(n,n\text{-}\pi^*,\pi^*)$ | (3,2,2,0,3,1,1,0) | (2,0,0,0,0,0,0,0) | 5.837 | **5.776** | **5.506**[c] | **5.986** | **5.993** | **5.896** | **5.826**[c] |

[a] Using reference (12e,12o) active space including full valence space. [b] Level shift = 0.4 au. [c] Level shift = 0.5 au.

**Table S12.** CASSCF, CASPT2, NEVPT2 and CASPT3/aug-cc-pVTZ vertical transition energies (eV) of Criegee's intermediate.

| State | Active space[a] (a',a") | State-average (A',A") | CASSCF | CASPT2 IPEA | CASPT2 NOIPEA | PC-NEVPT2 | SC-NEVPT2 | CASPT3 IPEA | CASPT3 NOIPEA |
|---|---|---|---|---|---|---|---|---|---|
| $^1A''(n\text{-}\pi^*)$ | (5,3) | (1,1) | 2.387 | **2.318** | **2.234** | **2.440** | **2.388** | **2.348** | **2.339** |
| $^1A'(\pi\text{-}\pi^*)$ | (5,3) | (2,0) | 4.201 | **3.881** | **3.645** | **3.746** | **3.866** | **3.870** | **3.825** |

[a] Using reference (10e,8o) active space including valence $\pi$, $\sigma_{OO}$, $\sigma_{CO}$, $\sigma^*_{OO}$, $\sigma^*_{CO}$, and one $n_O$ orbitals.

**Table S13.** CASSCF, CASPT2, NEVPT2 and CASPT3/aug-cc-pVTZ vertical transition energies (eV) of cyclobutadiene.

| State | Active space[a] ($a_g$,$b_{3u}$,$b_{2u}$,$b_{1g}$,$b_{1u}$,$b_{2g}$,$b_{3g}$,$a_u$) | State-average ($A_g$,$B_{3u}$,$B_{2u}$,$B_{1g}$,$B_{1u}$,$B_{2g}$,$B_{3g}$,$A_u$) | CASSCF | CASPT2 IPEA | CASPT2 NOIPEA | PC-NEVPT2 | SC-NEVPT2 | CASPT3 IPEA | CASPT3 NOIPEA |
|---|---|---|---|---|---|---|---|---|---|
| $^1A_g(\pi,\pi\text{-}\pi^*,\pi^*)$ | (2,2,2,2,1,1,1,1) | (2,0,0,0,0,0,0,0) | 4.217 | **4.039** | **3.971** | **4.056** | **4.086** | **4.041** | **4.031** |

[a] Using reference (12e,12o) active space including valence $\pi$, $\sigma_{CC}$, $\sigma^*_{CC}$ orbitals.

**Table S14.** CASSCF, CASPT2, NEVPT2 and CASPT3/aug-cc-pVTZ vertical transition energies (eV) of cyclopentadiene.

| State | Active space[a] ($a_1$,$b_1$,$b_2$,$a_2$) | State-average ($A_1$,$B_1$,$B_2$,$A_2$) | CASSCF | CASPT2 IPEA | CASPT2 NOIPEA | PC-NEVPT2 | SC-NEVPT2 | CASPT3 IPEA | CASPT3 NOIPEA |
|---|---|---|---|---|---|---|---|---|---|
| $^1A_1(\pi\text{-}\pi^*)$ | (0,2,0,2) | (2,0,0,0) | 6.609 | **6.686** | **6.249** | **6.817** | **6.848** | **6.650** | **6.558** |

[a] Using reference (4e,4o) active space including valence $\pi$ orbitals.

**Table S15.** CASSCF, CASPT2, NEVPT2 and CASPT3/aug-cc-pVTZ vertical transition energies (eV) of cyclopentadienethione.

| State | Active space ($a_1$,$b_1$,$b_2$,$a_2$) | State-average ($A_1$,$B_1$,$B_2$,$A_2$) | CASSCF | CASPT2 IPEA | CASPT2 NOIPEA | PC-NEVPT2 | SC-NEVPT2 | CASPT3 IPEA | CASPT3 NOIPEA |
|---|---|---|---|---|---|---|---|---|---|
| $^1B_1(n,\pi\text{-}\pi^*,\pi^*)$ | (0,4,1,2)[a] | (1,1,0,0) | 3.235 | **3.137** | **2.900** | **3.154** | **3.169** | **3.178** | **3.127** |
| $^1A_1(\pi\text{-}\pi^*)$ | (0,4,0,2)[b] | (2,0,0,0) | 5.572 | **5.418** | **4.919** | **5.428** | **5.466** | **5.423** | **5.340** |
| $^1A_1(n,n\text{-}\pi^*,\pi^*)$ | (0,4,1,2)[a] | (5,0,0,0) | 7.626 | **5.679** | **4.995** | **5.288** | **5.397** | **6.032** | **5.942** |
| $^3B_1(n,\pi\text{-}\pi^*,\pi^*)$ | (0,4,1,2)[a] | (1,1,0,0) | 3.210 | **3.105** | **2.867** | **3.121** | **3.136** | **3.140** | **3.087** |

[a] Using reference (8e,7o) active space including valence $\pi$ and $n_S$ orbitals. [b] Using reference (6e,6o) active space including valence $\pi$ orbitals.

**Table S16.** CASSCF, CASPT2, NEVPT2 and CASPT3/aug-cc-pVTZ vertical transition energies (eV) of cyclopentadienone.

| State | Active space ($a_1,b_1,b_2,a_2$) | State-average ($A_1,B_1,B_2,A_2$) | CASSCF | CASPT2 IPEA | CASPT2 NOIPEA | PC-NEVPT2 | SC-NEVPT2 | CASPT3 IPEA | CASPT3 NOIPEA |
|---|---|---|---|---|---|---|---|---|---|
| $^1B_1(n,\pi\text{-}\pi^*,\pi^*)$ | (0,4,1,2)[a] | (1,1,0,0) | 5.136 | **4.914** | **4.649** | **5.025** | **5.041** | **5.018** | **5.008** |
| $^1A_1(\pi,\pi\text{-}\pi^*,\pi^*)$ | (0,4,0,2)[b] | (2,0,0,0) | 6.146 | **5.983** | **5.612** | **6.022** | **6.057** | **5.979** | **5.910** |
| $^1A_1(\pi\text{-}\pi^*)$ | (0,4,1,2)[a] | (5,0,0,0) | 9.160 | **7.172** | **6.244** | **6.662** | **6.872** | **7.548** | **7.468** |
| $^3B_1(n,\pi\text{-}\pi^*,\pi^*)$ | (0,4,1,2)[a] | (1,1,0,0) | 5.075 | **4.814** | **4.542** | **4.913** | **4.933** | **4.913** | **4.897** |

[a] Using reference (8e,7o) active space including valence $\pi$ and $n_O$ orbitals. [b] Using reference (6e,6o) active space including valence $\pi$ orbitals.

**Table S17.** CASSCF, CASPT2, NEVPT2 and CASPT3/aug-cc-pVTZ vertical transition energies (eV) of diazete.

| State | Active space[a] ($a_g,a_u,b_u,b_g$) | State-average ($A_g,A_u,B_u,B_g$) | CASSCF | CASPT2 IPEA | CASPT2 NOIPEA | PC-NEVPT2 | SC-NEVPT2 | CASPT3 IPEA | CASPT3 NOIPEA |
|---|---|---|---|---|---|---|---|---|---|
| $^1A_g(\pi,\pi\text{-}\pi^*,\pi^*)$ | (4,2,4,2) | (3,0,0,0) | 7.081 | **6.699** | **6.584** | **6.649** | **6.732** | **6.684** | **6.672** |

[a] Using reference (12e,12o) active space including valence $\pi$, $\sigma_{CN}$, $\sigma^*_{CN}$ orbitals.

**Table S18.** CASSCF, CASPT2, NEVPT2 and CASPT3/aug-cc-pVTZ vertical transition energies (eV) of ethylene.

| State | Active space[a] ($a_g,b_{3u},b_{2u},b_{1g},b_{1u},b_{2g},b_{3g},a_u$) | State-average ($A_g,B_{3u},B_{2u},B_{1g},B_{1u},B_{2g},B_{3g},A_u$) | CASSCF | CASPT2 IPEA | CASPT2 NOIPEA | PC-NEVPT2 | SC-NEVPT2 | CASPT3 IPEA | CASPT3 NOIPEA |
|---|---|---|---|---|---|---|---|---|---|
| $^1A_g(\pi,\pi\text{-}\pi^*,\pi^*)$ | (1,1,1,1,0,0,0,0) | (2,0,0,0,0,0,0,0) | 14.119 | **13.163** | **13.093** | **13.109** | **13.262** | **13.205** | **13.177** |

[a] Using reference (4e,4o) active space including valence $\pi$, $\sigma_{CC}$, $\sigma^*_{CC}$ orbitals.

**Table S19.** CASSCF, CASPT2, NEVPT2 and CASPT3/aug-cc-pVTZ vertical transition energies (eV) of formaldehyde.

| State | Active space[a] ($a_1,b_1,b_2,a_2$) | State-average ($A_1,B_1,B_2,A_2$) | CASSCF | CASPT2 IPEA | CASPT2 NOIPEA | PC-NEVPT2 | SC-NEVPT2 | CASPT3 IPEA | CASPT3 NOIPEA |
|---|---|---|---|---|---|---|---|---|---|
| $^1A_1(n,n\text{-}\pi^*,\pi^*)$ | (2,2,1,0) | (3,0,0,0) | 12.225 | **10.420** | **10.400** | **10.265** | **10.296** | **10.713** | **10.718** |

[a] Using reference (6e,5o) active space including valence $\pi$, $n_O$, $\sigma_{CO}$, $\sigma^*_{CO}$ orbitals.

**Table S20.** CASSCF, CASPT2, NEVPT2 and CASPT3/aug-cc-pVTZ vertical transition energies (eV) of glyoxal.

| State | Active space[a] ($a_g,a_u,b_u,b_g$) | State-average ($A_g,A_u,B_u,B_g$) | CASSCF | CASPT2 IPEA | CASPT2 NOIPEA | PC-NEVPT2 | SC-NEVPT2 | CASPT3 IPEA | CASPT3 NOIPEA |
|---|---|---|---|---|---|---|---|---|---|
| $^1A_g(n,n\text{-}\pi^*,\pi^*)$ | (4,2,4,2) | (2,0,0,0) | 5.924 | **5.372** | **5.211** | **5.518** | **5.546** | **5.535** | **5.549** |

[a] Using reference (14e,12o) active space including valence $\pi$, $n_O$, $\sigma_{CC}$, $\sigma_{CO}$, $\sigma^*_{CC}$, $\sigma^*_{CO}$ orbitals.

**Table S21.** CASSCF, CASPT2, NEVPT2 and CASPT3/aug-cc-pVTZ vertical transition energies (eV) of hexatriene.

| State | Active space[a] ($a_g$,$a_u$,$b_u$,$b_g$) | State-average ($A_g$,$A_u$,$B_u$,$B_g$) | CASSCF | CASPT2 IPEA | CASPT2 NOIPEA | PC-NEVPT2 | SC-NEVPT2 | CASPT3 IPEA | CASPT3 NOIPEA |
|---|---|---|---|---|---|---|---|---|---|
| $^1A_g(\pi\text{-}\pi^*)$ | (0,3,0,3) | (2,0,0,0) | 5.618 | **5.571** | **5.171** | **5.636** | **5.667** | **5.556** | **5.472** |

[a] Using reference (6e,6o) active space including valence π orbitals.

**Table S22.** CASSCF, CASPT2, NEVPT2 and CASPT3/aug-cc-pVTZ vertical transition energies (eV) of naphthalene.

| State | Active space[a] ($a_g$,$b_{3u}$,$b_{2u}$,$b_{1g}$,$b_{1u}$,$b_{2g}$,$b_{3g}$,$a_u$) | State-average ($A_g$,$B_{3u}$,$B_{2u}$,$B_{1g}$,$B_{1u}$,$B_{2g}$,$B_{3g}$,$A_u$) | CASSCF | CASPT2 IPEA | CASPT2 NOIPEA | PC-NEVPT2 | SC-NEVPT2 | CASPT3 IPEA | CASPT3 NOIPEA |
|---|---|---|---|---|---|---|---|---|---|
| $^1A_g(\pi\text{-}\pi^*)$ | (0,0,0,0,3,2,3,2) | (3,0,0,0,0,0,0,0) | 6.895 | **6.793** | **5.942**[b] | **6.900** | **6.958** | **6.809** | **6.748**[b] |

[a] Using reference (10e,10o) active space including valence π orbitals. [b] Level shift = 0.4 au.

**Table S23.** CASSCF, CASPT2, NEVPT2 and CASPT3/aug-cc-pVTZ vertical transition energies (eV) of nitrosomethane.

| State | Active space[a] (a',a") | State-average (A',A") | CASSCF | CASPT2 IPEA | CASPT2 NOIPEA | PC-NEVPT2 | SC-NEVPT2 | CASPT3 IPEA | CASPT3 NOIPEA |
|---|---|---|---|---|---|---|---|---|---|
| $^1A'(n,n\text{-}\pi^*,\pi^*)$ | (7,2) | (2,0) | 4.966 | **4.787** | **4.775** | **4.794** | **4.815** | **4.748** | **4.742** |

[a] Using reference (12e,9o) active space including all valence orbitals but the $\sigma_{CH}$ and $\sigma^*_{CH}$.

**Table S24.** CASSCF, CASPT2, NEVPT2 and CASPT3/aug-cc-pVTZ vertical transition energies (eV) of nitrous acid.

| State | Active space (a',a") | State-average (A',A") | CASSCF | CASPT2 IPEA | CASPT2 NOIPEA | PC-NEVPT2 | SC-NEVPT2 | CASPT3 IPEA | CASPT3 NOIPEA |
|---|---|---|---|---|---|---|---|---|---|
| $^1A'(n,n\text{-}\pi^*,\pi^*)$ | (10,3)[a] | (3,0) | 8.185 | **7.967** | **7.970** | **8.001** | **7.992** | **7.939** | **7.945** |
| | (11,3)[b] | (4,0) | 8.337 | **8.005** | **7.978** | **8.009** | **8.025** | **7.969** | **7.968** |

[a] Using reference (18e,13o) active space including full valence space. [b] Using reference (18e,14o) active space including full valence space and one Rydberg 3s orbital.

**Table S25.** CASSCF, CASPT2, NEVPT2 and CASPT3/aug-cc-pVTZ vertical transition energies (eV) of nitroxyl.

| State | Active space[a] (a',a") | State-average (A',A") | CASSCF | CASPT2 IPEA | CASPT2 NOIPEA | PC-NEVPT2 | SC-NEVPT2 | CASPT3 IPEA | CASPT3 NOIPEA |
|---|---|---|---|---|---|---|---|---|---|
| $^1A'(n,n\text{-}\pi^*,\pi^*)$ | (7,2) | (2,0) | 4.670 | **4.366** | **4.358** | **4.371** | **4.398** | **4.364** | **4.361** |

[a] Using reference (12e,9o) active space including full valence space.

**Table S26.** CASSCF, CASPT2, NEVPT2 and CASPT3/aug-cc-pVTZ vertical transition energies (eV) of octatetraene.

| State | Active space[a] $(a_g,a_u,b_u,b_g)$ | State-average $(A_g,A_u,B_u,B_g)$ | CASSCF | CASPT2 IPEA | CASPT2 NOIPEA | PC-NEVPT2 | SC-NEVPT2 | CASPT3 IPEA | CASPT3 NOIPEA |
|---|---|---|---|---|---|---|---|---|---|
| $^1A_g(\pi\text{-}\pi^*)$ | (0,4,0,4) | (2,0,0,0) | 4.879 | **4.741** | **4.326** | **4.783** | **4.814** | **4.751** | **4.680** |

[a] Using reference (8e,8o) active space including valence $\pi$ orbitals.

**Table S27.** CASSCF, CASPT2, NEVPT2 and CASPT3/aug-cc-pVTZ vertical transition energies (eV) of oxalyl fluoride.

| State | Active space[a] $(a_g,a_u,b_u,b_g)$ | State-average $(A_g,A_u,B_u,B_g)$ | CASSCF | CASPT2 IPEA | CASPT2 NOIPEA | PC-NEVPT2 | SC-NEVPT2 | CASPT3 IPEA | CASPT3 NOIPEA |
|---|---|---|---|---|---|---|---|---|---|
| $^1A_g(n,n\text{-}\pi^*,\pi^*)$ | (4,2,4,2) | (2,0,0,0) | 9.044 | **8.814** | **8.643** | **8.942** | **8.958** | **8.899** | **8.923** |

[a] Using reference (14e,12o) active space including valence $\pi$, $n_O$, $\sigma_{CC}$, $\sigma_{CO}$, $\sigma^*_{CC}$, $\sigma^*_{CO}$ orbitals.

**Table S28.** CASSCF, CASPT2, NEVPT2 and CASPT3/aug-cc-pVTZ vertical transition energies (eV) of pyrazine.

| State | Active space $(a_g,b_{3u},b_{2u},b_{1g},b_{1u},b_{2g},b_{3g},a_u)$ | State-average $(A_g,B_{3u},B_{2u},B_{1g},B_{1u},B_{2g},B_{3g},A_u)$ | CASSCF | CASPT2 IPEA | CASPT2 NOIPEA | PC-NEVPT2 | SC-NEVPT2 | CASPT3 IPEA | CASPT3 NOIPEA |
|---|---|---|---|---|---|---|---|---|---|
| $^1A_g(n,n\text{-}\pi^*,\pi^*)$ | (1,2,0,1,1,2,0,1)[a] | (3,0,0,0,0,0,0,0) | 8.094 | **7.845** | **7.584** | **8.037** | **8.067** | **7.945** | **7.949** |
| $^1A_g(\pi\text{-}\pi^*)$ | (0,2,0,1,0,2,0,1)[b] | (2,0,0,0,0,0,0,0) | 8.423 | **8.712** | **8.163** | **8.948** | **9.005** | **8.667** | **8.616** |
| | (1,2,0,1,1,2,0,1)[a] | (3,0,0,0,0,0,0,0) | 8.436 | **8.746** | **8.208** | **8.999** | **9.051** | **8.676** | **8.624** |

[a] Using reference (10e,8o) active space including valence $\pi$ and $n_N$ orbitals. [b] Using reference (6e,6o) active space including valence $\pi$ orbitals.

**Table S29.** CASSCF, CASPT2, NEVPT2 and CASPT3/aug-cc-pVTZ vertical transition energies (eV) of tetrazine.

| State | Active space[a] $(a_g,b_{3u},b_{2u},b_{1g},b_{1u},b_{2g},b_{3g},a_u)$ | State-average $(A_g,B_{3u},B_{2u},B_{1g},B_{1u},B_{2g},B_{3g},A_u)$ | CASSCF | CASPT2 IPEA | CASPT2 NOIPEA | PC-NEVPT2 | SC-NEVPT2 | CASPT3 IPEA | CASPT3 NOIPEA |
|---|---|---|---|---|---|---|---|---|---|
| $^1A_g(n,n\text{-}\pi^*,\pi^*)$ | (1,2,1,1,1,2,1,1) | (2,0,0,0,0,0,0,0) | 5.419 | **4.566** | **4.318** | **4.608** | **4.688** | **4.917** | **4.951** |
| $^1B_{3g}(n,n\text{-}\pi^*,\pi^*)$ | (1,2,1,1,1,2,1,1) | (1,0,0,0,0,0,1,0) | 6.590 | **5.853** | **5.218** | **6.149** | **6.200** | **6.201** | **6.215** |
| $^3B_{3g}(n,n\text{-}\pi^*,\pi^*)$ | (1,2,1,1,1,2,1,1) | (1,0,0,0,0,0,1,0) | 6.562 | **5.388** | **4.861** | **5.506** | **5.570** | **5.829** | **5.848** |

[a] Using reference (14e,10o) active space including valence $\pi$ and $n_N$ orbitals.
